# Supplementary material for: Soft regression trees: a model variant and a decomposition training algorithm
Source: arXiv:2501.05942 source file (2025-01-27)
Supplement: Supplementary file 1 [file EC_initialization_procedure.tex]

\section{Initialization procedure scheme}\label{appendix:Init_procedure}
\textcolor{black}{Since formulation \eqref{eq:obj} is highly nonconvex, the solution found by state-of-the-art nonlinear optimization solvers turns out to be very sensitive to the starting points. An appropriate choice of starting points can enhance the training phase and lead to solutions with a better testing accuracy.}

\textcolor{black}{Our initialization procedure is based on the idea of recursively clustering the input vectors associated to each data point in a number of clusters corresponding to the number of leaf nodes. Starting from the root node with a single cluster composed of all data points, we recursively split the current cluster into two sub-clusters so as to have for each leaf node at depth $D$ a distinct cluster.}

\textcolor{black}{Given a current node $t$, for simplicity of notation let $I_t$ denote the set of indices of data points falling in this node. Then, $I_{left_t}$ and $I_{right_t}$ which are the sets of the indices of data points assigned to its left and right children nodes are determined by clustering $I_t$ into two clusters. This procedure ensures that clustering at each node is applied only after having applied it to its ancestor node.}

\textcolor{black}{Since the solution of clustering method depends on random seed, the initialization procedure is repeated $\bm{r}$ times. In our work, we use the well-known \textbf{K-means} algorithm \cite{lloyd1982least} with \textit{K-means++} random initialization \cite{arthur2007k}.} 

\textcolor{black}{For each $j = 1,\dots,\bm{r}$, let $A_{\tau_L}^j$ denote the assignment of the training data points to the clusters associated to the leaf nodes, that is obtained by applying the clustering method from the root to the bottom. To assess the goodness of the assignment $A_{\tau_L}^j$, a silhouette score $Sil(A_{\tau_L}^j)$ is computed. The assignment with the best silhouette score is selected for the initialization.}

\textcolor{black}{Silhouette scores are measures which express how close (similar) each data point is with respect to the other data points within its cluster compared to the ones of the neighboring clusters \cite{dudek2020silhouette}. In our implementation we consider as silhouette score the Davies-Bouldin index \cite{davies1979cluster} which expresses the average similarity measure of each cluster with its most similar cluster.}

The general scheme of the initialization procedure is reported below. It is important to notice that for both the clustering method and silhouette score several alternatives can be considered.

 %RIMUOVE IL NUMERO
\begin{algorithm}[H]
\floatname{algorithm}{} %PER RIMUOVERE ALGORITHM
\caption{}
\label{alg:init}
$\bm{Input}:\, dataset\, \bm{I};\, depth \,\bm{D}; \,repetitions\, \bm{r}.\\\bm{Output}:\,assignment\,with\,data\,points\,\,associated\,\,to\,\,leaf\,\,nodes\,\,{\hat{A}_{\tau_L}^{j}}. $
  
  {\fontsize{10}{12}\selectfont
  \begin{algorithmic}[1]
    \Procedure{InitializationProcedure}{$\bm{I},\bm{D},\bm{r}$}
    
    \State $DB^{*} \gets BigM$ \Comment{setting an initial big value for the best Davies-Bouldin index}
    	\For{$ j = 1,...,\bm{r} $}\Comment{loop over the repetitions}
    	\State $A_{\tau_L}^j \gets \{\emptyset\}$
    	
    		\For{$t = 1,...,|\tau_B|$}\Comment{loop over the branch nodes}
    		\State $\textrm{generate } I_{left_{t}} \textrm{and } I_{right_{t}} \textrm{by applying K-means with 2 clusters}$
    		\If{$t \;\textrm{belongs to the } D-1 \textrm{level of tree}$} 
    		\State $A_{\tau_L}^j \gets A_{\tau_L}^j \cup \{I_{left_{t}}\} \cup \{I_{right_{t}}\} $
    		\EndIf
    		\EndFor
    		
    	\State $DB \gets Davies-Bouldin(A_{\tau_L}^j)$
    	\If{$DB < DB^{*}$}
    	      \State $DB^{*} \gets DB$
    	      \State ${\hat{A}_{\tau_L}^{j}} \gets A_{\tau_L}^j$

    	\EndIf
    	
    	\EndFor
    \State \textbf{return} ${\hat{A}_{\tau_L}^{j}}$
    \EndProcedure
  \end{algorithmic}
  }
\end{algorithm}
