# Supplementary material for: Soft regression trees: a model variant and a decomposition training algorithm
Source: arXiv:2501.05942 source file (2025-01-27)
Supplement: Supplementary file 2 [file EC_preliminary.tex]

\section{Preliminary experiments}
\label{ec:preliminary_ex}
In this appendix, we summarize preliminary experiments to assess the potential impact of the data points reassignment heuristics coupled with the NODEC-DR decomposition algorithm. First, we present results obtained on a synthetic dataset to illustrate the possible benefits of the data points reassignment heuristic described in Section \ref{subsec:implementation}. Then, we make a performance comparison between the plain optimization (i.e. optimize the overall objective function with an off-the-shelf solver), the plain decomposition method, and decomposition combined with the reassignment heuristic, using four representative datasets.

For all the experiments the performance are evaluated by means of a k-fold cross validation with k = 4 and for each fold 20 distinct starting points are generated either randomly.

\textcolor{black}{To assess the ability of the decomposition algorithm with the reassignment heuristic to improve the routing of the data points from the root along the tree, as compared to the plain decomposition, we consider a synthetic dataset.} The synthetic dataset is composed by $p=3$ predictor variables and 1500 data points structurally clustered into four clusters. Each distinct cluster can be identified by one of the four leaf nodes of a tree at $D=2$. Figure \ref{fig:b} shows the 3D plot for the input vectors, while for the output
response each leaf has associated a distinct linear regression whose coefficients are given in the following matrix:
$$\begin{bmatrix}
    -1.51 & 0.46 & -3.81 \\
    2.32 & -1.41 & -0.11\\
    -1.56 & 1.12 & 1.53\\
    -2.32 & 1.41 & 0.11
\end{bmatrix}
$$
where the rows represent the leaf nodes and the columns the coefficients of the variables. We also apply a white noise of zero mean 0.1 standard deviation.

\begin{figure}[H] 
\centering
        \includegraphics[width=0.5\textwidth]{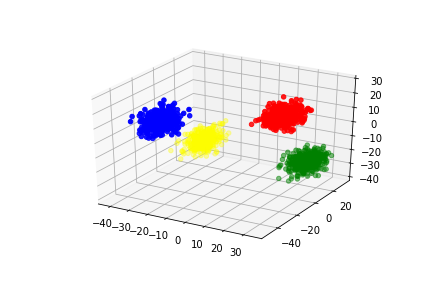}%
    \caption{3D representation of the 4 clusters of the synthetic dataset.}\label{fig:b}
\end{figure}

\textcolor{black}{Figure \ref{fig:gini} shows the Gini index distribution for both the plain decomposition and the decomposition with the reassignment heuristic on the synthetic dataset. Since we know which cluster each data point belongs to, the Gini index helps us determine which method routes data points more accurately towards the leaf node associated to its cluster. Clearly, the decomposition with the data points reassignment heuristic turns out to be more effective in routing data points to their respective leaf nodes compared to plain decomposition, often achieving a Gini index of zero (i.e. indicating a perfect routing).}

\begin{figure}[H]
\vspace{1pt}
    \centering
    \includegraphics[width=0.5\textwidth]{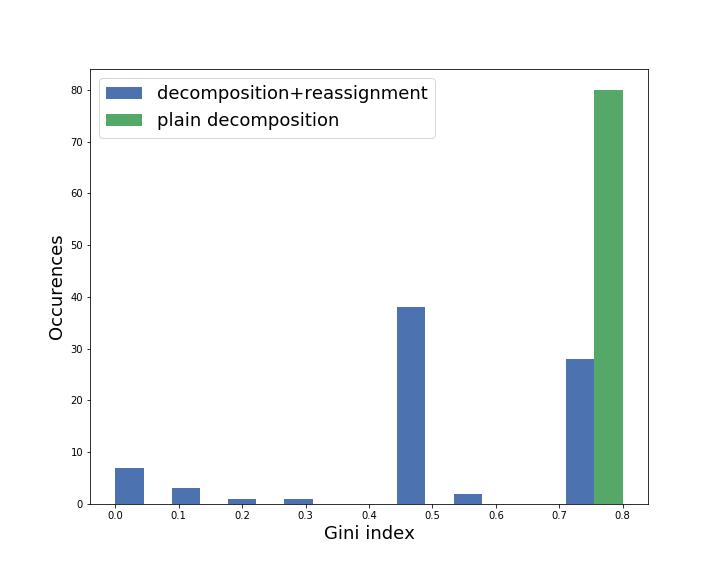}
    \caption{Histogram of the distributions of the Gini index value on different runs for plain decomposition (green) and decomposition with data points reassignment heuristic (blue).}
    \label{fig:gini}
\end{figure}

\textcolor{black}{A second set of experiments was conducted on four representative datasets of different sizes, to compare plain model optimization (without decomposition) with incremental introduction of decomposition and the data points reassignment heuristic. Table \ref{table:confrontoalgo} reports the performance in terms of average testing $R^2$, standard deviation $\sigma$, computational time, and the number of times when a very weak model with negative $R^2$ (i.e. when the prediction is worse than the simple average) is obtained.}

\textcolor{black}{It is easy to see that a plain decomposition method significantly reduces training times compared to plain optimization, but inclusion of the reassignment heuristics improves substantially the testing accuracy, keeping training times low. For instance, in the airfoil-self-noise dataset, there is an improvement in the accuracy of over $20\%$, while for the puma dataset, the improvement exceeds $50\%$, all while keeping training times low.}

\begin{table}[h]
\centering
\resizebox{1\columnwidth}{!}{
\begin{tabular}{lcccccccc}
\cline{2-9}
                                             & \multicolumn{4}{c}{housing}                                                               & \multicolumn{4}{c}{airfoil-self-noise}                                                    \\ \cline{2-9} 
                                             &  $R^2$  & $\sigma$   & time (sec)                & $R^2<0$              &  $R^2$  & $\sigma$   & time (sec)                & $R^2<0$              \\ \hline
plain optimization                      & 0.7142               & 0.0553               & 6.326                & 0                    & 0.5126               & 0.0153               & 2.62                & 1                    \\
plain decomposition                      & 0.7143               & 0.0553               & 1.04                 & 0                    & 0.512                & 0.0157               & 2.35                 & 0                    \\
decomposition+reassignment                            & 0.8094               & 0.088               & 1.79                 & 0                    & 0.7354               & 0.0538               & 3.34                 & 0                    \\
                                             & \multicolumn{1}{l}{} & \multicolumn{1}{l}{} & \multicolumn{1}{l}{} & \multicolumn{1}{l}{} & \multicolumn{1}{l}{} & \multicolumn{1}{l}{} & \multicolumn{1}{l}{} & \multicolumn{1}{l}{} \\ \cline{2-9} 
                                             & \multicolumn{4}{c}{ailerons}                                                              & \multicolumn{4}{c}{puma}                                                                  \\ \cline{2-9} 
                                             &  $R^2$  & $\sigma$   & time (sec)                & $R^2<0$              &  $R^2$  & $\sigma$   & time (sec)                & $R^2<0$              \\ \hline
plain optimization                      & 0.8112               & 0.00594              & 537.6              & 40                   & 0.2157               & 0.03069              & 67.9                & 1                    \\
plain decomposition                      & 0.8227               & 0.0044               & 24.72                 & 20                   & 0.2152               & 0.031                & 23.7                & 0                    \\
decomposition+reassignment                           & 0.8324               & 0.0078               & 15.62                & 0                    & 0.7352               & 0.1336               & 39.45               & 0                    \\
\end{tabular}
}
\caption{Results in terms of testing $R^2$, standard deviation $\sigma$, computing time and number of negative $R^2$ for 4 datasets (airfoil, ailerons, housing and puma). Each row represents the steps taken from the first (optimization with a off the shelf solver) to the last (our decomposition method with reassignment and initialization procedure)}
\label{table:confrontoalgo}
\end{table}

Finally, to assess the effectiveness of the initialization procedure with the selection of the best Davies-Bouldin index, the algorithm \ref{alg:init} is applied to the housing dataset (results are similar for the other datasets). A simple linear regression is fitted to the 80 results where the response is the testing $R^2$ and the predictor variable is the silhouette score associated to each initialization. The regression results in Figure \ref{fig:statisticainizializzazione} show a strong negative correlation between the silhouette score and the testing $R^2$, as indicated by the high significance and the negative sign of the regression coefficient. Note that the lower the Davies-Bouldin index the higher the quality of the clustering.

\begin{figure}[H]
\vspace{1pt}
\centering
\includegraphics[width=0.7\linewidth]{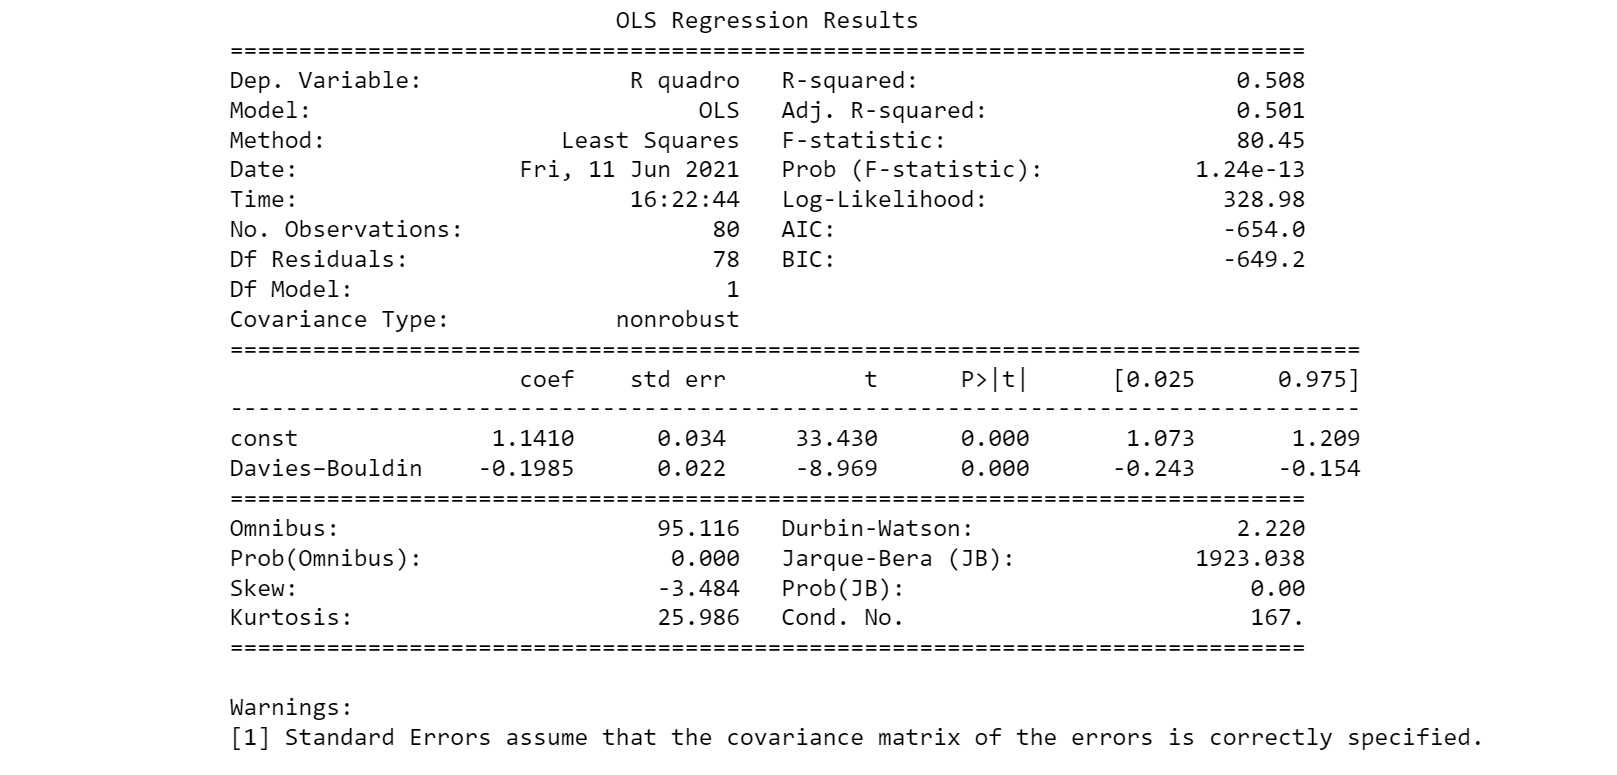}
\caption{Results obtained for the housing dataset by fitting a linear regression to assess the relation between the testing $R^2$ (response) and the Davies-Bouldin score associated to each initialization (independent variable) generated by our initialization procedure.}
\label{fig:statisticainizializzazione}
\end{figure}
