# Supplementary material for: Soft regression trees: a model variant and a decomposition training algorithm
Source: arXiv:2501.05942 source file (2025-01-27)
Supplement: Supplementary file 3 [file appen2.tex]

\section{Experiment details}
In the following subsections, details on experimental setup used are reported.

\subsection{Experimental Platform}
The experiments are carried out on a PC with Intel(R) Core(TM) i7-9700K CPU @ 3.60GHz with 16GB RAM.

\subsection{Model implementations and software packages}
\begin{itemize}
    \item \textbf{MRRT}: The MRRT formulation have been implemented in Python 3.6.10. The tree structure is built in the Cython, a C extension for python. For the optimization of the leaf nodes variables we used the \texttt{scipy.sparse} 1.5.2. For the optimization of the branching nodes variables, in the case of generic optimization, we use the SLSQP solver in \texttt{scipy.optimize} 1.5.2 package in tandem with \texttt{numba} 0.51.2 while for the weighted logistic regression we used the logistic regression model from  \texttt{sklearn} 0.23.1 package with default parameters setting.
    \item \textbf{ORT-L}: We used OptimalTreeRegressor in version 2.0.2 of Interpretable AI package (IAI) (https://docs.interpretable.ai/stable/). We were given a free license for this software. Source code was not available.
    \item \textbf{ORRT}: We followed the instructions given by the authors in Section 4.1 of \cite{blanquero2022sparse}. The model has been implemented using the \texttt{scipy.optimize} 1.5.2 package in Python 3.6.10 in tandem with \texttt{numba} 0.51.2 and the SLSQP method.
    \item \textbf{HME}: We used the implementation of the EM algorithm for the HME in \texttt{smt} 2.0 package \cite{SMT2ArXiv} for python with the default parameter setting and assuming the least square as expert associated to each leaf node. 
    \item \textbf{RF}: We used the \texttt{randomForest} package \cite{rcolorbrewer2018package} in R 4.0.1 with the default parameter setting.
\end{itemize}
