# Supplementary material for: Soft regression trees: a model variant and a decomposition training algorithm
Source: arXiv:2501.05942 source file (2025-01-27)
Supplement: Supplementary file 4 [file appen6.tex]

\section{Fairness constraints: experimental setting and datasets}\label{appendix:MRRT_HME}

To assess the efficiency of the  \textit{predictive parity} and \textit{accuracy assurance} constraints the MRRT trees are evaluated by means of k-fold cross-validation, with k = 5 and depth $D = 2$. Testing $R^2$ and the \textit{predictive parity} are computed as the average obtained over all 5 folds. In this case we do not apply our starting point strategy, and for each fold the trees are built from 5 different random starting solutions.

For the experiments on \textit{predictive parity} constraints we used the datasets Boston Housing, MEPS and LSAC. 
As to Boston Housing, as in \cite{blanquero2021sparse}, we assume that the sensitive group $G$ is composed by individuals above the third quartile of predictor variable  \textit{black proportion of population}. 

The MEPS dataset represents a large-scale surveys of families, where each observation contains total expenditures of an individual as well as number of other variables describing his or her demographic and socio-economic status. In this case we consider the $race$ predictor variable as the sensitive variable for the group $G$. 

As to LSAC dataset, this dataset is composed of the results of a classifier that must predict whether a student will pass a test based on the law school admissions test score (LSAT) and the undergraduate GPA. For this dataset we consider the $race$ predictor variable as the sensitive variable for the group $G$.

\begin{figure}[h]
    \centering
    \includegraphics[width=0.6\linewidth]{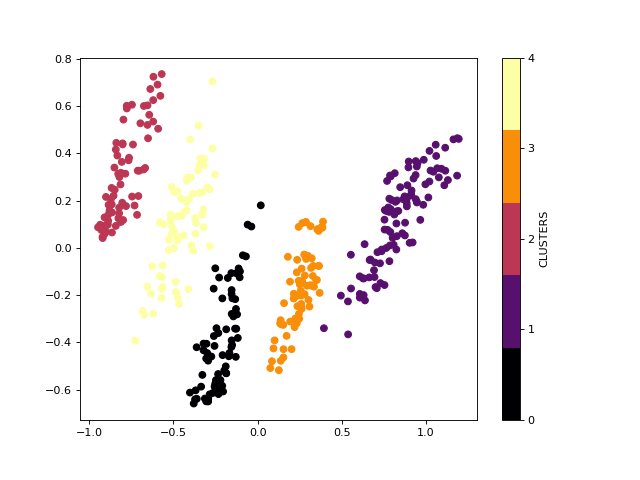}
    \caption{PCA with the first two principal components for the Auto-mpg dataset.}
    \label{fig:PCA-auto}
\end{figure}
Concerning the \textit{accuracy assurance} constraint on the Auto-mpg dataset, we artificially created a sensitive group.

Applying PCA on the entire dataset, it is possible to distinguish 5 distinct clusters on the first two principal components, as shown in Figure \ref{fig:PCA-auto}. To do so, we trained the model without any constraint on the entire dataset and selected a subset of individuals ($10\%$) from the cluster with the highest residuals. From this cluster we consider the individuals with higher residual as the sensitive group. This allowed us to select the instances on which to apply the constraint \eqref{eq:accu_ass1}.

        \begin{figure}
\centering
     %\textbf{Overall}\par\medskip
     \includegraphics[width=0.7\linewidth]{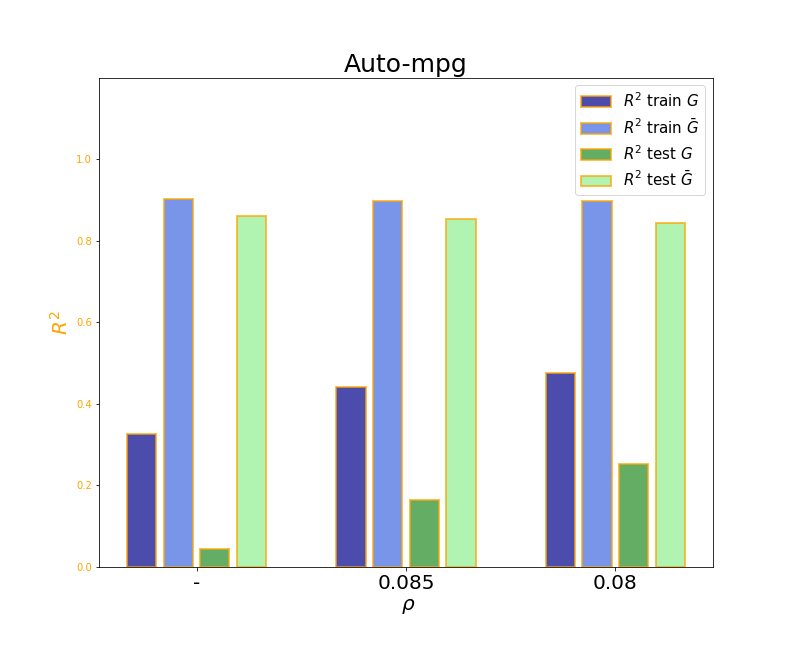}
   \caption[]{Results of MRRT model with \textit{accuracy assurance} constraint \eqref{eq:accu_ass1}. The blue bar represents the results on the training set while the green one the results on the test set. }
   \label{fig:accuracyassurance}

\end{figure}
