# Supplementary material for: Soft regression trees: a model variant and a decomposition training algorithm
Source: arXiv:2501.05942 source file (2025-01-27)
Supplement: Supplementary file 5 [file hme.tex]

\section{Comparison with Hierarchical Mixture of Experts}\label{appendix:MRRT_HME}
In this Appendix we present the comparative results for the 15 datasets of the MRRT $\ell_2$ and HMEs with trees of depth $D=2,3$, following the experimental setting detailed in Section \ref{sec:experiments_regression}. For the HME training, we used the \texttt{smt} 2.0 package \cite{SMT2ArXiv}, assuming the least square as expert associated to each leaf node. 

Table \ref{tab:HME} reports the testing $R^2$, the standard deviation $\sigma$, Anomalie for the number of times where the solver of HME failed to find a solution, and the computational time in seconds. The rows marked with a dash indicate instances where the solver failed to find a solution in any of the 80 runs. The Averages reported do not consider datasets where HME failed to give any solution.

\begin{table}[h!]
\caption{Comparison of MRRT $\ell_2$ ORRT model on 15 datasets in terms of out-of-sample $R^2$, standard deviation $\sigma$ (to be multiplied by $1e^{-2}$). Averages (with an asterisk) do not consider datasets where HME failed to give any solution.}\label{tab:HME}
\resizebox{\textwidth}{!}{
\begin{tabular}{lccccccc|ccccccc}
\hline
          & \multicolumn{7}{c|}{D=2}                                                             & \multicolumn{7}{c}{D=3}                                                           \\ \cline{2-15} 
Dataset   & \multicolumn{3}{c}{MRRT $\ell_2$}   & \multicolumn{4}{c|}{HME}                       & \multicolumn{3}{c}{MRRT $\ell_2$}  & \multicolumn{4}{c}{HME}                      \\ \cline{2-15} 
          & $R^2$ & $\sigma (1e^{-2})$ & Time   & $R^2$ & $\sigma (1e^{-2})$ & Time   & Anomalie & $R^2$ & $\sigma(1e^{-2})$ & Time   & $R^2$ & $\sigma(1e^{-2})$ & Time  & Anomalie \\ \hline
Abalone   & 0.554 & 2.14               & 8.74   & 0.541 & 4.7                & 0.38   & 2        & 0.564 & 2.16              & 23.97  & 0.527 & 4.06              & 1.85  & 37       \\
Ailerons  & 0.836 & 0.56               & 18.95  & 0.821 & 1.01               & 6.33   & 40       & 0.835 & 0.43              & 50.48  & 0.819 & 1.17              & 12.25 & 77       \\
Airfoil   & 0.748 & 2.9                & 5.16   & 0.613 & 2.9                & 0.6116 & 0        & 0.807 & 2.14              & 11.35  & 0.643 & 3.42              & 0.98  & 1        \\
Auto mpg  & 0.87  & 2.37               & 2.47   & 0.85  & 3.6                & 0.165  & 38       & 0.873 & 2.17              & 6.15   & -     & -                 & -     & 80       \\
Compact   & 0.98  & 0.168              & 37.17  & 0.981 & 0.18               & 8.01   & 0        & 0.98  & 0.27              & 72.72  & 0.982 & 0.12              & 9.61  & 0        \\
Computer  & 0.964 & 2.49               & 1.99   & -     & -                  & -      & 80       & 0.955 & 3.37              & 4.03   & -     & -                 & -     & 80       \\
Cpu small & 0.969 & 0.23               & 31.34  & 0.971 & 0.2                & 2.06   & 0        & 0.97  & 0.25              & 58.67  & 0.972 & 0.2               & 4.9   & 0        \\
Delta     & 0.701 & 0.63               & 10.4   & 0.693 & 0.89               & 0.83   & 0        & 0.706 & 1                 & 29.53  & 0.689 & 1.6               & 2.23  & 0        \\
Elevators & 0.871 & 0.47               & 39.55  & 0.832 & 0.47               & 7.91   & 0        & 0.884 & 0.57              & 94.66  & 0.846 & 0.62              & 17.02 & 21       \\
Friedman  & 0.894 & 0.85               & 134.46 & 0.918 & 0.25               & 21.96  & 0        & 0.938 & 0.28              & 311.76 & 0.944 & 0.21              & 50.5  & 0        \\
Housing   & 0.846 & 3.4                & 2.92   & 0.761 & 7.9                & 0.57   & 0        & 0.872 & 4.48              & 7.35   & 0.741 & 0.09              & 0.58  & 66       \\
Kin8nm    & 0.723 & 2.28               & 19.02  & 0.734 & 1.4                & 3.3    & 0        & 0.786 & 1.9               & 50.73  & 0.811 & 1.2               & 4.54  & 0        \\
Lpga2009  & 0.891 & 2.58               & 2.23   & -     & -                  & -      & 80       & 0.877 & 2.5               & 4.96   & -     & -                 & -     & 80       \\
Puma      & 0.815 & 0.9                & 44.95  & 0.641 & 6.7                & 11.83  & 0        & 0.883 & 0.88              & 136.51 & 0.866 & 1.2               &     28.24  &  16   \\
Yacht     & 0.976 & 0.77               & 2.49   & 0.705 & 15.04              & 0.2    & 0        & 0.983 & 0.48              & 5.41   & 0.459 & 14.2              & 0.23  & 43       \\ \hline

\multicolumn{1}{c}{AVG ARIT*}                                                    & 0.829 & 1.36          & 27.5  & 0.774 & 3.48        & 4.93  & -     & 0.851 & 1.237            & 71.09       & 0.775 & 2.34         & 9.52  &   -         \\ \hline
\multicolumn{1}{c}{AVG GEO*}                                                    & 0.82 & 0.94          & 14.07  & 0.763 & 1.51         & 1.83  & -     & 0.841 & 0.81            & 39.41       & 0.756 & 0.853         & 3.57  &   -         \\ \hline
\end{tabular}
}

\end{table}

Overall, for both depths $D=2$ and $D=3$, the results exhibit similarities in terms of both accuracy and computational time. 

Concerning the testing $R^2$, MRRT $\ell_2$ exhibits better performance compared to HME in most of the datasets. In particular, excluding the datasets where HME failed to find a solution, MRRT $\ell_2$ achieves better results on 9 out of 13 datasets for depth $D=2$, and on 8 out of 12 datasets for depth $D=3$. Moreover, MRRT $\ell_2$ is able to reach a level of testing $R^2$ up to $27\%$ higher, whereas in the 3 cases where HME performs better, the difference is not more than $2.5\%$.  

As to the computational time HME tends to exhibit faster performance, but typically less than one order of magnitude. It is worth noting that, as shown by the last rows where the average performance are reported, the advantage in terms of the computational time of HMEs appears not significant when compared to the testing $R^2$ improvement achieved by MRRT $\ell_2$.
