# Supplementary material for: Soft regression trees: a model variant and a decomposition training algorithm
Source: arXiv:2501.05942 source file (2025-01-27)
Supplement: Supplementary file 7 [file appendix_preliminary.tex]

\section{Additional material related to preliminary experiments}\label{appendix:preliminary}

\textcolor{red}{This Appendix provides details on the generation of the synthetic dataset used in Subsection \ref{sec:preliminary_ex} and an experiment on the effectiveness of our initialization procedure.}

The synthetic dataset is composed by $p=3$ predictor variables and 1500 data points structurally clustered into four clusters
so that, in principle, each distinct cluster can be identified by one of the four leaf nodes of a tree at depth 2. Figure \ref{fig:b} shows the 3D plot for the input vectors, while for the output
response each leaf has associated a distinct linear regression whose coefficients are given in the following matrix:
$$\begin{bmatrix}
    -1.51 & 0.46 & -3.81 \\
    2.32 & -1.41 & -0.11\\
    -1.56 & 1.12 & 1.53\\
    -2.32 & 1.41 & 0.11
\end{bmatrix}
$$
where the rows represent the leaf nodes and the columns the coefficients of the variables. We also apply a white noise of zero mean 0.1 standard deviation.

\begin{figure}[H] 
\centering
        \includegraphics[width=0.6\textwidth]{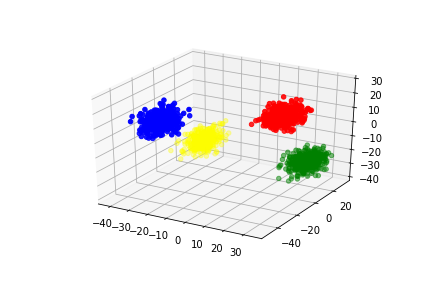}%
    \caption{3D representation of the 4 clusters of the synthetic dataset.}\label{fig:b}
\end{figure}

Concerning the evaluation of the initialization procedure, to assess the effectiveness of it with the selection of the best Davies-Bouldin index, the algorithm \ref{alg:init} and decomposition method are applied to the Housing dataset (results are similar for the other datasets). Then a simple linear regression is fitted to the 80 results where the response is the testing $R^2$ and the predictor variable is the silhouette score associated to each initialization. 

The regression results in Figure \ref{fig:statisticainizializzazione} show a strong negative correlation between the silhouette score and testing $R^2$, as indicated by the high significance and the negative sign of the regression coefficient. Note that the lower is the Davies-Bouldin index the better is the quality of the clustering.

\begin{figure}[H]
\centering
\includegraphics[width=0.7\linewidth]{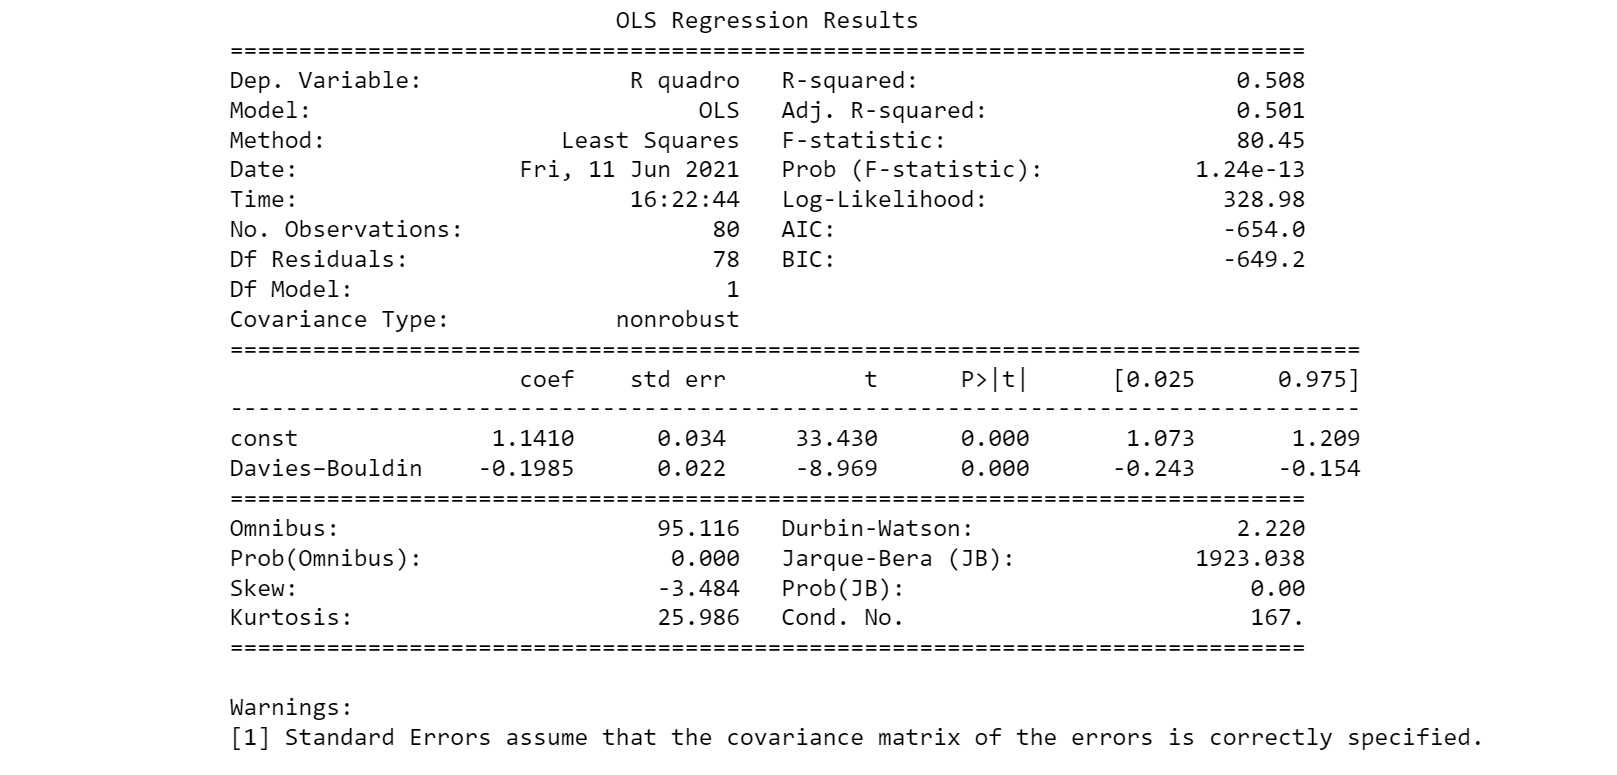}
\caption{Results obtained on the housing dataset by fitting a linear regression to assess the relation between the testing $R^2$ (response) and the Davies-Bouldin score associated to each initialization (independent variable) generated by our initialization procedure.}
\label{fig:statisticainizializzazione}
\end{figure}
